# Supplementary material for: Online Min-Max Paging
Source: arXiv:2212.03016 source file (2022-12-06)
Supplement: Supplementary file 1 [file appendix.tex]

% This is an alternative presentation of the online convex programming framework and the upper bound on paging, meant as an alternative version to insert after section 3. 

% \section{Extending the \cite{azarOnlineAlgorithms2016} Framework}

% We extend the framework of \cite{azarOnlineAlgorithms2016} by adding box constraints on the variables for a specific set of constraint matrices $A$ and cost vectors $b$. In other words, we solve the following problem \mh{what are the input parameters}:

% \begin{equation*}
%     \begin{array}{lll}
%         \text{minimize } & f(x) &  \\
%         \text{subject to } & A x \le D - k \ones \\
%         & 0 \le x_i \le 1 & \forall i \in [I], \\
%     \end{array}
% \end{equation*}
% where $A \in \{0,1\}^{T \times I}$, $I \in \N$ is the number of variables, $T \in \N$ is the number of rounds, $k \in \N$ is a fixed constant we call the \emph{slack} of the program and $D$ is a vector containing in its $t$th entry the number of non-zero entries in row $t$ of $A$. We let $d = \max_{t \in [T]} D_t$ denote the maximum row sparsity of $A$. 

% We let $A$ be the constraint matrix described above, and we will employ an online primal-dual approach in order to arrive at a competitive fractional algorithm. The following will be our convex dual:
% \begin{equation*}
%     \begin{array}{ll}
%         \text{maximize } & D(y,z) = \sum_{t=1}^T (D_t - k) y_t - \sum_{i \in [I]} z_i - f^*(A^\top y - z), \\
%         \text{subject to }
%         &\begin{array}{ll} 0 \le y_t &  \forall t \in [T]\\
%          0 \le z_i & \forall i \in [I]\\
%         \end{array}
%     \end{array}
% \end{equation*}
% where $f^*(y) = \sup_{w \in \R_+^I} \left( \langle w, y \rangle - f(w) \right)$ is the conjugate function. We only use the dual for the analysis of our algorithm in order to lower bound OPT, hence we can assume that we know the whole matrix $A$ and all of the variables $y_t$ and $z_i$. We write $y$ and $z$ for the vectors of these variables respectively, with $y$ being ordered in order of increasing $t$ and $z$ being ordered the same way as $x$. Before moving on, we need the following observation:

% \begin{obs}\label{o0}
% The conjugate function $f^*(v): \R_{\ge 0}^I \to \R$ of a convex function $f$ is monotonically increasing in $v$.
% \end{obs}
% \begin{proof}
% Indeed, let $c \in \R_{\ge 0}^I$, then
% \[
% f^*(v) = \sup_{w \in \R_{\ge 0}^I} \langle v, w \rangle - f(w) \le \sup_{w \in \R_{\ge 0}^I} \langle v, w \rangle + \langle c, w \rangle - f(w) = f^*(v + c),
% \]
% as $\langle c, w\rangle$ is always non-negative.
% \end{proof}

% \begin{rem}
% From now on, we assume that the target function $f(x)$ is convex, monotone, differentiable and $f(0)=0$. Furthermore we require that $\nabla f(x)$ is monotonically nondecreasing in every coordinate, i.e. for every coordinate $i \in I$ we have $(\nabla f(x))_i \ge (\nabla f(x'))_i$ for any two vectors $x \ge x'$.
% \end{rem}

% As duality in convex optimization is not as straightforward as in the linear setting, we need the following:

% \begin{lem}[Weak Duality]
% For any feasible $x \in [0,1]^I$ and $y, z \in \R_{\ge0}^I$, we have 
% \begin{equation*}
%     f(x) \ge \sum_{t \in [T]} (D_t-k) y_t - \sum_{i \in [I]} z_i - f^*(A^\top y - z).
% \end{equation*}
% \end{lem}
% \begin{proof}
% As $x$ is feasible, it must satisfy $A x \ge D - k \ones$, which gives $D - k \ones - Ax \le \zeros$, and similarly, from $x \le \ones$ we get $x - \ones \le \zeros$. Thus taking the inner product of these vectors with the non-negative vectors $y$ and $z$ respectively will yield a negative number, and hence we get the first inequality in the following chain of inequalities:
% \begin{align*}
%     f(x) &\ge f(x) + y^\top (D -k \ones - Ax) + z^\top (x - \ones) \\
%     &= \sum_{t \in [T]} (D_t - k)y_t - \sum_{i \in [I]} z_i - (y^\top Ax - z^\top x - f(x))\\
%     &= \sum_{t \in [T]} (D_t - k)y_t - \sum_{i \in [I]} z_{i} - (\langle A^\top y - z, x\rangle - f(x))\\
%     &\ge \sum_{t \in [T]} (D_t - k)y_t - \sum_{i \in [I]} z_{i} - \sup_{w \in \R_+^T} (\langle A^\top y - z, w\rangle - f(w))\\
%     &= \sum_{t \in [T]} (D_t - k)y_t - \sum_{i \in [I]} z_{i} - f^*(A^\top y - z).\\
% \end{align*}
% All equalities are obtained from simple rearrangement of terms and the final inequality is due to the definition of the supremum.
% \end{proof}

% We now extend the algorithm of \cite{azarOnlineAlgorithms2016}, which did not allow upper bounds on the variables. This leads to Algorithm \ref{fractional}. 

% The algorithm is based on a continuous time $\tau$ which initially is $0$ and increases throughout the algorithm's processing of the constraints. As all variables start at $0$ when they are introduced and increase at a rate dependent on $\tau$, we can write $x_{i}(\tau)$, $y_t(\tau)$ and $z_{i}(\tau)$ to express the value of the variables as a function of $\tau$.

% Furthermore, we let $\tau(t)$ denote the value of $\tau$ after we finish processing the $t$th constraint. Note that, by the algorithm $\tau(0) = 0$.

% The algorithm uses parameters $r$ and $s_{i}(\tau)$ which are to be determined later. Note that $s_{i}(\tau)$ depends on the value of $\tau$ and $i$ and hence is not a constant parameter.

% \begin{algorithm}
% \caption{A fractional algorithm for fair paging}\label{fractional}
% \begin{algorithmic}
% \Require $r > 0$ and $s_{i}(\tau) > 0$, $s_{i}(\tau)$ monotonically decreasing in $\tau$
% \State $\tau \gets 0$
% \For{each round $t \in [T]$}
% \State if $x_i$ has not been seen before let $x_{i}(\tau) \gets 0$ and $z_i(\tau) \gets 0$
% \State $y_t(\tau) \gets 0$
% \While{$A_t x < D_t - k$}
%     \State increase $\tau$ uniformly at rate $1$
%     \State increase $y_t(\tau)$ uniformly at rate $r$
%     \For{all $x_i$ with $a_{ti} = 1$ in parallel}
%     \If{$x_{i} < 1$}
%         \State increase $x_{i}(\tau)$ at rate $s_{i}(\tau) \left(x_{i}(\tau) + \frac{1}{d}\right)$
%     \Else
%         \State increase the corresponding $z_{i}(\tau)$ at rate $r$
%     \EndIf
%     \EndFor
% \EndWhile
% \EndFor
% \end{algorithmic}
% \end{algorithm}

% \begin{obs}\label{o1}
% We have $y_t(\tau(t-1)) = 0$ for all $t \in [T]$.
% \end{obs}
% \begin{proof}
% By the algorithm, $y_t$ is initialized to $0$ at the time $\tau$ we start processing the constraint revealed in round $t$, which is equal to $\tau(t-1)$ as we do not increase $\tau$ in between rounds.
% \end{proof}

% From now on let $t(i)$ denote the first round $t$ in which $x_i$ appears with a non-zero coordinate and let $t'(i)$ denote the round it last appears. $t(i)$ is the first round in which $x_i$ will be increased by Algorithm \ref{fractional}. Furthermore, we let $T(i) = \{t \in [T] \mid a_{ti} > 0\}$ be the set of rounds in which $x_i$ can possibly be increased.

% \begin{lem}\label{xlowerbound}
% Let  $\bar{x}$ denote the value of $x$ after the algorithm has processed all constraints in $A$ and similarly for $\bar{y}$ and $\bar{z}$. If $s_{i}(\tau)$ is monotonically decreasing in $\tau$, then
% \begin{equation}\label{lem2eq}
%     \bar{x}_{i} \ge \frac1d \left(\exp \left( \frac{ s_{i}'}{r} \left( \sum_{t \in T(i)} \bar{y}_t - \bar{z}_{i} \right) \right)  - 1\right),
% \end{equation}
% where $s_{i}' = s_{i}(\tau(t'(i)))$. This is the minimal value that $s_{i}(\tau)$ takes on while $x_{i}(\tau)$ is being increased by our algorithm.
% \end{lem}
% \begin{proof}
% We will show that the Lemma holds for any $\tau$ and the corresponding $x_{i}(\tau)$, $y_t(\tau)$, $z_{i}(\tau)$ produced by the algorithm. Let 
% \[\tau_{i}' = \min \left(\{\tau > \tau(t(i) - 1) \mid x_{i}(\tau) = 1\} \cup \{\tau(t'(i))\} \right),
% \]
% i.e. the smallest $\tau$ for which $x_{i}(\tau) = 1$ if it exists, or $\tau(t'(i))$ otherwise. 

% Let us fix $i$ and consider the case $\tau < \tau_{i}'$. In this case, by the definition of the growth rates in the algorithm, we get the following differential equation if we consider $x_{i}(\tau)$ as a function of $y_t(\tau)$ for any $t$ such that $t \ge t(i)$ and $\tau \le \tau_{i}'$ if $t \in T(i)$:
% \[
% \frac{dx_{i}}{dy_t} = \frac{s_{i}(\tau)}{r} \left(x_{i} + \frac1d \right).
% \]
% If $t \notin T(i)$ then $x_i(\tau)$ will not increase during the round and we are done.

% Taking $s_{i}'$ as above, we turn this into the inequality
% \[
% \frac{dx_{i}}{dy_t} \ge \frac{s_{i}'}{r} \left(x_{i} + \frac1d \right),
% \]
% which we can solve using a standard separation of variables approach. Let $\tau''(t) = \min(\tau(t), \tau_{i}')$. Integrating over the interval $[\tau(t-1), \tau''(t)]$, which is the only interval during which both $y_t$ and $x_{i}$ can increase, gives 
% \begin{equation}\label{lem2basic}
% \ln\left(x_{i} + \frac1d \right) \biggr\vert_{\tau(t-1)}^{\tau''(t)} \ge \frac{s_{i}'}{r} y_t \biggr\vert_{\tau(t-1)}^{\tau''(t)}.
% \end{equation}
% Expanding this expression gives
% \[
% \ln \left(x_{i}(\tau''(t)) + \frac1d \right) - 
% \ln \left(x_{i}(\tau(t-1)) + \frac1d \right) \ge \frac{s_{i}'}{r} (y_t(\tau''(t)) - y_t(\tau(t-1)),
% \]
% which, using Observation \ref{o1}, gives 
% \[
% \ln \left(x_{i}(\tau''(t)) + \frac1d \right) - 
% \ln \left(x_{i}(\tau(t-1)) + \frac1d \right) \ge \frac{s_{i}'}{r} y_t(\tau''(t)),
% \]
% and we note that if $\tau(t) \ge \tau''(t)$ then $y_t(\tau(t)) = \bar{y}_t$, as it will no longer increase.

% Summing over all rounds $t$ such that $a_{ti} = 1$ and $t \le t'' = \min \{t \in [T] \mid x(\tau(t)) = 1\}$ gives
% \[
% \sum_{t \in T(i) \setminus [t'' + 1, T]} \left( \ln \left(x_{i}(\tau''(t)) + \frac1d \right) - \ln \left(x_{i}(\tau(t-1)) + \frac1d \right) \right) \ge \frac{s_{i}'}{r} \sum_{t \in T(i) \setminus [t'' + 1, T]} \bar{y}_t + y_{t'}(\tau_{i}').
% \]
% The left sum is telescoping, as $x_i(\tau)$ will not increase for rounds in which $a_{ti} = 0$, and we note that $x_i(\tau(t(i) - 1) = 0$. Thus the above expression can be simplified to
% \begin{equation*}
% \ln \left(x_{i}(\tau_{i}')) + \frac1d \right) - \ln \left( \frac1d \right) \ge \frac{s_{i}'}{r} \sum_{t \in T(i) \setminus [t'' + 1, T]} \bar{y}_t + y_{t'}(\tau_{i}').
% \end{equation*}

% In the case $\tau_{i}' = \tau(t'(i))$ we are done, as $z_{i}$ is never increased and hence by taking exponentials and rearranging we obtain the statement of the lemma with $\bar{z}_{i} = 0$. Otherwise, we want to consider $\tau > \tau_{i}'$. In this case we know that $x_{i}(\tau) = 1$ and the algorithm increases $z_{i}(\tau)$ rather than $x_{i}(\tau)$. This means the left hand side of Inequality \eqref{lem2basic} is no longer increasing while the right hand side term is still increasing. 

% In order for the inequality to continue to hold, we subtract $\frac{s_{i}'}{r} z_{i}(\tau)$ from the right hand side in order to counteract the increase of $y_t(\tau)$, yielding 
% \begin{equation}\label{lem2eq2}
% \ln \left(x_{i}(\tau) + \frac1d \right) - \ln \left( \frac1d \right) \ge \frac{s_{i}'}{r} \left( \sum_{t \in T(i) \setminus [\hat t, T] } \bar{y}_t + y_{\hat{t}}(\tau) - z_{i}(\tau)\right).
% \end{equation}

% During a round $\hat t$ and time $\tau$ where $x_{i}(\tau) = 1$, $z_{i}(\tau)$ increases at rate $r$, which cancels out the increase of $y_{\hat t}(\tau)$, as the rate of change, i.e. the derivative, becomes
% \[
% \frac{d}{d\tau}\frac{s_{i}'}{r} \left( \sum_{t \in T(i) \setminus [\hat{t}, T]} \bar{y}_t + y_{\hat{t}}(\tau) - z_{i}(\tau)\right) = \frac{s_{i}'}{r} (r - r) = 0.
% \]
% Thus Inequality \eqref{lem2eq2} continues to hold as $\tau$ increases even while $x_{i}(\tau)$ remains constant at $1$.

% The increase in $z_{i}(\tau)$ counteracts all increase in the right hand side from the time $\tau''(t'')$, where $x_{i}(\tau)$ becomes $1$, until time $\tau(t'(i))$ whence $z_{i}(\tau)$ will stay constant, thus we have $\bar{z}_{i} = z_{i}(\tau(t'(i))$.

% Finally, after examining the inequality for $\tau \ge \tau(t'(i))$ the expression becomes 
% \begin{equation*}
% \ln \left(d \bar{x}_{i} + 1 \right)\ge \frac{s_{i}'}{r} \left( \sum_{t \in T(i)} \bar{y}_t - \bar{z}_{i} \right),
% \end{equation*}
% which gives the lemma after taking exponentials and rearranging.
% \end{proof}

% This immediately implies the following:

% \begin{claim}\label{feasibility}
% The $x(\tau(t))$ produced by Algorithm \ref{fractional} throughout its execution are feasible for the primal for all $t \in [T]$ and the vector $(A^\top \bar{y} - \bar{z})_{i} \le \frac{r}{s_{i}'} \ln(d+1)$.
% \end{claim}
% \begin{proof}
% The first statement follows via the definition of the algorithm immediately from the fact that we can always fulfill the primal constraints, for example by setting all the variables to $1$.

% To show the second statement, we note that $\bar{x} \le \mathbf{1}$, which with Equation \eqref{lem2eq} gives us
% \[
%     \frac1d \left(\exp \left( \frac{ s_{i}'}{r} \left( \sum_{t \in T(i)} \bar{y}_t - \bar{z}_{i} \right) \right)  - 1\right) \le \bar{x}_{i} \le 1.
% \]
% Taking the left- and right-hand sides, after rearranging and taking logarithms gives us
% \[
% \sum_{t \in T(i)} \bar{y}_t - \bar{z}_{i}  \le \frac{r}{s_{i}'} \ln(d + 1),
% \]
% where the left-hand side is $(A^T \bar{y} - \bar{z})_{i}$.
% \end{proof}

% \begin{obs}
% The function $s_{i}(\tau) = \frac{\partial f(x(\tau))}{\partial x_{i}}^{-1}$ is monotonically decreasing in $\tau$.
% \end{obs}
% \begin{proof}
% This immediately follows from the fact that we require the gradient to be non-decreasing in each coordinate.
% \end{proof}

% For the final theorem we need to define $q$, the \emph{polynomial growth} of a function, which is defined as the smallest integer such that for all $x \in \R_{\ge 0}^T$,
% \[
% \langle \nabla f(x), x \rangle \le q f(x).
% \]

% \begin{thm}\label{thm:frac}
% After processing the sequence $\sigma$, Algorithm \ref{fractional} produces an $O((k q \log(d+1))^q)$ competitive solution $\bar{x}$ for fractional fair paging with an objective function that has polynomial growth $q$, if we set $s_{i}(\tau) = \frac{\partial f(x)}{\partial x_{i}}^{-1}$ and $r = \frac{\delta}{\ln(d+1)}$ where $\delta$ will be determined in the proof.
% \end{thm}
% \begin{proof}
% By weak duality, it suffices to show that the primal is no larger than $O((k q \log(d+1))^q)$ times the dual which is a lower bound on OPT by weak duality.

% We will now bound the growth rates of the primal and dual for each round $t$ in terms of $\tau$. It suffices to only consider the case $A_t x(\tau) < D_t - k$, as otherwise, nothing needs to be done.

% Let 
% \[
% C_t(\tau) = \{ i \mid t \in T(i) \text{ and } x_{i}(\tau) < 1 \}
% \]
% be the set of indices of variables $x_{i}(\tau)$ at round $t$ which are increasing. 

% Similarly, let 
% \[
% D_t(\tau) = \{ i \mid t \in T(i) \text{ and } x_{i}(\tau) = 1 \}
% \]
% be the set of indices of the variables $x_{i}(\tau)$ which are no longer increasing. Note that $|C_t(\tau)| + |D_t(\tau)| = D_t \le d$, by definition of $D$. 

% While processing the $t$th constraint, we have, by the choice of $s_{i}(\tau)$, and the fact that $x_{i}(\tau)$ is constant if $i \in D_t(\tau)$:
% \begin{align*}
%     G_1 \coloneqq \frac{df(x)}{d\tau} = \sum_{i \in [I]} \frac{\partial f(x)}{\partial x_{i}} \frac{\partial x_{i}(\tau)}{\partial \tau}  &= \sum_{i \in [I]} \frac{\partial f(x)}{\partial x_{i}} \left( s_{i}(\tau) \left(x_{i}(\tau) + \frac1d \right) \right) \\
%     &= \sum_{i \in C_t{(\tau)}} \left(x_{i}(\tau) + \frac1d \right) \le |C_t(\tau)| + 1.
% \end{align*}
% The first equality is due to the chain rule for vector-valued functions, while the last inequality follows as there are no more than $d$ pages in $C_t(\tau)$ at any time, hence the second term in the summation sums to at most $1$ and each $x_{i}(\tau) \le 1$.

% For the linear term $\sum_{t \in [T]} (D_t-k)y_t(\tau) - \sum_{i \in [I]} z_{i}(\tau)$ in the dual, we find that, in round $t$, as $y_t$ may only increase during that round, and the fact that both $\frac{dy_t(\tau)}{d\tau} = r$ and $\frac{dz_{i}(\tau)}{d\tau} = r$ if $i \in D_t(\tau)$,
% \begin{align*}
% G_2 \coloneqq \frac{d \sum_{t} (D_t-k)y_t(\tau) - \sum_{i} z_{i}(\tau)}{d\tau} = (D_t - k) r - \sum_{i \in D_t(\tau)} r = r (D_t - k - |D_t(\tau)|).
% \end{align*}

% The ratio $\frac{D_t - k - |D_t(\tau)|}{|C_t(\tau)|+1} = \frac{|C_t(\tau)| - k}{|C_t(\tau)|+1} = 1 - \frac{k}{|C_t(\tau)|+1}$ is minimized when $|C_t(\tau)| = k+1$, as (1) it is monotonically increasing in $|C_t(\tau)|$ and (2) $|C_t(\tau)| > k $, since otherwise $A_t x(\tau) > |D_t(\tau)| = D_t - |C_t(\tau)| \ge D_t - k$, contradicting our initial assumption. Thus the minimum of $\frac{D_t - k - |D_t(\tau)|}{|C_t(\tau)|+1}$  is $\frac{1}{k+1}$ and the ratio between the growth rates of the primal and the linear term of the dual is bounded from below by 
% \[
% \frac{G_2}{G_1} \ge \frac{r}{k+1}.
% \]
% As both functions start from $0$ at time $\tau = 0$, their values after processing all elements are also bounded by this ratio as our primal never grows faster than the linear term times this ratio. Thus with our choice of $r$ it follows that 
% \[
% \sum_t (D_t-k) \bar{y}_t - \sum_{i} \bar{z}_{i} \ge
% \frac{\delta}{(k+1)\ln(d+1)} f(\bar x)
% \]
% %Finally, from the fact that $x_{p,j} \le 1$ we get that 
% %\[
% %\frac1n \left(\exp \left( \frac{ s_{p}'}{r} \left( \sum_{t = t(p, j)+1}^{t(p,j+1)-1} y_t - z_{p,j} \right) %\right)  - 1\right) \le 1,
% %\]
% %which, after rearranging yields
% %\[
% %\sum_{t = t(p, j)+1}^{t(p,j+1)-1} y_t - z_{p,j} \le r \frac{\partial f(\bar x)}{\partial x_{p,j}} \ln(n + 1).
% %\]
% %The choice for $s_p'$ is justified as $\nabla f(x)$ is monotonically increasing, since $f(x)$ is convex.
% % clear up this sentence
% Plugging 
% $s_{i}(\tau) = \frac{\partial f(x)}{\partial x_{i}}^{-1}$ and $r = \frac{\delta}{\ln(d+1)}$ 
% %our choice of $s_{p,j}(\tau)$ and $r$ 
% into the second statement of Claim \ref{feasibility}, we obtain that $A^T y - z \le \delta \nabla f(\bar{x})$, which allows us to bound the conjugate term of the dual as
% \[
% f^*(A^T \bar y - \bar z) \le f^*(\delta \nabla f(\bar x)) \le 
% \begin{cases}
% \delta^{\frac{q}{q-1}} \cdot (q - 1) \cdot f(\bar x) & \text{ if $q > 1$},\\
% 0 & \text{ if $q = 1$},
% \end{cases}
% \]
% where the second inequality uses Lemma 4 of \cite{azarOnlineAlgorithms2016} and the first inequality is due to Observation \ref{o0}.
% Hence the relationship between the final value $D(\bar y, \bar z)$ of the dual and the final value $f(\bar x)$ of the primal is
% \[
% D(\bar y, \bar z) = \sum_t (D_t - k) \bar{y}_t - \sum_{i} \bar{z}_{i} - f^*(A^T \bar y - \bar z) \ge 
% \left( \frac{\delta}{(k+1) \ln(1+n)} - \delta^{\frac{q}{q-1}} \cdot (q - 1)\right) \cdot f(\bar x).
% \]
% The term $\left( \frac{\delta}{(k+1) \ln(1+n)} - \delta^{\frac{q}{q-1}} \cdot (q - 1)\right)$ is a polynomial in $\delta$. It is maximized for $\delta = \frac{1}{((k+1) \ln(n + 1) q)^{q-1}}$ giving a competitive ratio of $\frac{1}{((k+1) q \ln(n+1))^q}$,  which is positive for $n\ge 2$. Hence, by rearranging and weak duality we obtain 
% \[
% f(\bar{x}) \le \left((k+1) q \ln(n+1) \right)^q D(\bar y, \bar z) \le \left((k+1) q \ln(n+1) \right)^q f(\OPT).
% \]
% \end{proof}

% \begin{rem}
% It is often the case that $\nabla f(0) = 0$ but $\nabla f(x) > 0$ everywhere else in $\R_+^I$. In this case we start the algorithm at $\epsilon \ones$ for some sufficiently small $\epsilon$ to avoid the division by $0$.
% \end{rem}

% 

% 

% 

% 

% \section{Fractional Fair Paging}

% In order to obtain an upper bound for fair paging, we consider a fractional relaxation. This lets us formulate fair paging as an online convex programming problem. We begin by fixing some notation.

% From now let $p$ be a variable representing a page, let $t$ be a variable representing a particular round, and let $j$ be a variable representing the $j$th time a page was requested. We use the variables $x_{p,j}$ in place of $x_i$.

% Furthermore, we let $r(p,t)$ indicate the number of requests to page $p$ up to and including round $t$ and let $t(p,j)$ be the time at which the page $p$ is requested for the $j$th time. Any variable with a bar denotes the final value of the variable, once the algorithm has finished processing it, as $\bar{x}$ above.

% With this notation in hand, we can state the following convex programming formulation for paging:

% \begin{equation*}
%     \begin{array}{lll}
%         \text{minimize } & f(x) &  \\
%         \text{subject to } & \sum_{p \in P \setminus \{p_t\}} x_{p, r(p,t)} \ge |B(t)| - k & \forall t \in [T] \\
%         & 0 \le x_{p,j} \le 1 & \forall p \in [n], j \in [r(p,T)] \\
%     \end{array}
% \end{equation*}

% The variables $x_{p,j}$ are bounded between $0$ and $1$ and indicate the fractional amount of page $p$ that has been removed from the cache after it was added at time $t(p,j)$, in the same manner as in the LP relaxation of the classical paging problem. Once the page is requested again at time $t(p,j+1)$ we have to move the $\bar{x}_{p,j}$ fraction of the page that has been ejected since that request back into the cache, increasing the $p$th entry of the cost vector by that amount. 

% The covering constraint $\sum_{p \in P \setminus \{p_t\}} x_{p,r(p,t)} \ge |B(t)| - k$ indicates that once we finish processing the $t$th round, we must have ejected at least $|B(t)| - k$ fractional page mass from the cache, or, equivalently, we have at most $k$ fractional mass in the cache.

% When processing a round, we are given a new variable $x_{p_t,j}$, which is initialized to 0, corresponding to the $j$th request to page $p_t$, together with the constraint $\sum_{p \in P \setminus \{p_t\}} x_{p, r(p,t)} \ge |B(t)| - k$ and a box constraint for variable $x_{p,j}$. 
% We note that a variable $x_{p,j}$ will only appear in the constraints corresponding to rounds $t \in [t(p,j)+1, t(p,j+1)-1]$. Once a constraint has been revealed, we need to increase some of the variables $x_{p,r(p,t)}$ for $p \in P \setminus \{p_t\}$ until it is satisfied. When the constraint corresponding to round $t$ is satisfied, we are presented with the next page $p_{t+1}$ and its corresponding constraint. 

% Given a request sequence, we can define a constraint matrix $A \in \{0,1\}^{T \times T}$ as
% \[
% A_{t,(p,j)} = \delta_{p,j}(t),
% \]
% where
% \[
% \delta_{p,j}(t) = 
% \begin{cases}
% 1 & \text{if $t \in [t(p,j)+1, t(p,j+1) - 1]$}\\ 
% 0 & \text{otherwise.}
% \end{cases}
% \]
% Note that in round $t$ we can determine all non-zero entries as they only depend on the variables encountered up to round $t$. The columns corresponding to future variables are implicitly set to $0$.

% At this point we note that the matrix $A$ is a $0-1$ matrix of maximal sparsity $n-1$, allowing us to use the online convex programming framework we have developed.

% %\begin{proof}
% %We claim that the gradient of a convex function is monotonically increasing in each $x_{p,j}(\tau)$. Once this is established, the observation follows immediately from the definition of $s_{p,j}(\tau)$.
% %
% %Now, by the definition of a convex, differentiable function $g(w)$ we have
% %\[
% %g(w) \ge g(z) + \langle \nabla g(z), w - z \rangle,
% %\]
% %for any vectors $w$ and $z$ in its domain. Hence, we also have 
% %\[
% %g(z) \ge g(w) + \langle \nabla g(w), z - w \rangle,
% %\]
% %and by adding the two inequalities, we get
% %\begin{equation}\label{o7}
% %0 \le \langle \nabla g(w) - \nabla g(z), w - z \rangle.
% %\end{equation}
% %
% %Now consider vectors $y$ and $y'$ where $y' = y + c \cdot e_m$, where $e_m$ is the $m$th standard basis vector and $c > 0$ is a constant. Using Inequality \eqref{o7} we find that $0 \le \langle \nabla g(y') - \nabla g(y), c \cdot e_m \rangle$, which gives $\frac{\partial g} {\partial y_m}(y) \le \frac{\partial g}{\partial y_m}(y')$ by the fact that $c > 0$. As $m$ was arbitrary, the claim follows.
% %\end{proof}

% To obtain the target function we need the cost vector $\mathbf{c}(t)$. We obtain it if we sum the costs $x_{p,j}(\tau(t))$ for each page $p$. To this end we define a matrix $C \in \{0,1\}^{n \times T}$ such that the $p$-th row of $C$ contains a $1$ in column $(p,j)$ for each of the variables $x_{p,j}$ for $j \in [r(p,T)]$ and $0$ otherwise.
% It follows that $C \cdot x(\tau(t)) = \mathbf{c}(t)$ for all $t \in [T]$. Note that the solution of the fractional fair paging problem can be determined by setting $f(x)$ to $\|C x \|_\infty$.

% However, we find that $\|\cdot \|_\infty$ is not differentiable in $\R_{\ge 0}^T$ and so we cannot apply the framework directly to 
% $\|C x \|_\infty$. Thus, instead we run the above algorithm with
% $f(x) :=\|C x \|_{\log n}^{\log{n}}.$ 
% This is a polynomial in the variables of $x$ with maximum degree $\log n$, hence $q = \log n$. We further note that the gradient of this function is monotonous in the sense that for any $x'$ and $x$ where $x'$ is pointwise greater than $x$ we have $\nabla f(x') > \nabla f(x)$ pointwise as well.

% Note that $\|C x \|_{\log n}^{\log n}$ produces an $n$-approximation of
% $\|C x \|_\infty^{\log n}$ as shown by the next lemma, which states a well-known fact about  norms in finite-dimensional vector spaces.

% 
% \begin{lem}
% For any vector $x \in \R^n$,
% \[
% \|x\|_\infty \le \|x\|_{\log n} \le e \|x\|_\infty.
% \]
% \end{lem}
% \begin{proof}
% The first inequality is trivial. To obtain the second, note
% \[
% \|x\|_{\log n}^{\log n} = \sum_{i = 1}^n |x_i|^{\log n} \le n \cdot \max_{i \in [n]}{|x_i|^{\log n}} = n \|x\|_\infty^{\log n}
% \]
% which, after taking roots gives the result, as $n^{\frac{1}{\log n}} = e$.
% \end{proof}
% Let $x^*$ denote the optimum solution for the problem with $\ell_{\infty}$-norm. 
% Thus, from Theorem~\ref{thm:frac} it follows that
% $$\| x^*\|_{\infty}^{\log n} \le \| x^*\|_{\log n}^{\log n} 
% \le \| {\bar x}\|_{\infty}^{\log n} = P(\bar x) 
% \le (( k+1) \log^2 (n +1))^{\log n} \| x^*\|_{\log n}^{\log n} \le n (( k+1) \log^2 (n +1))^{\log n} \| x^*\|_{\infty}^{\log n}.$$
% Applying the $\log n$-th root shows that $P(\bar x)^{1/\log n}$ gives an 
% $O(k \log^2 n)$-approximation to the optimum solution.
%  
% %  (Note that $\|Cx\|_{\log n}^m$ is not differentiable at $0$ for any $m < \log n$, so we can not simply choose $m = O(1)$ to remove a $\log$-factor, unless we are fine without differentiability at $0$ (probably the case))

% \begin{cor}
% There exists a $O(k \log^2 n)$ competitive algorithm for fractional fair paging.
% \end{cor}

%%% Local Variables:
%%% mode: latex
%%% TeX-master: "main"
%%% End:
